# Supplementary material for: Using Anomaly Feature Vectors for Detecting, Classifying and Warning of Outlier Adversarial Examples
Source: arXiv:2107.00561 source file (2021-07-01)
Supplement: Supplementary file 1 [file 18_appendix_cluster_groups.tex]

% \section{Clustering of Similar Attacks}
% \subsection{Cluster Groups}
% Because perturbations induced by different attacks are ultimately very similar, in order to produce reliable attack classifications, we cluster similar attacks into groups and classify the membership of a sample into such clusters. Our approach can classify an adversarial sample into one of such attack cluster/groups. We propose and demonstrate the clustering of similar attack classes based on a transitive closure with respect to FPR and FNR values. This technique allows to tailor the FPR or FNR response of the network as well as increase overall detection rates.
